# Supplementary material for: Computing the Haar state of $\mathcal{O}(SL_q(3))$ using value preserving (anti)homomorphisms
Source: arXiv:2401.08614 source file (2024-04-26)
Supplement: Supplementary file 1 [file appendix_C.tex]

\section{Useful equations} \label{apd:c}
When we switch the order of high complexity segments\\ with $ceg$ segment:
\begin{equation}
\begin{split}
    cegaek &= aekceg+(q^3 - q)*afhceg-(q - 1/q)*bdkceg-(q^2 - 1)^2/q*bfgcdh,\\
    cegafh &= q^2*afhceg+(1 - q^2)*bfgcdh,\\
    cegbdk &= q^{-2}*bdkceg+(1 - q^{-2})*bfgcdh,
    \label{apeq:1}
\end{split}
\end{equation}
with $cdh$ segment:
\begin{equation}
    \begin{split}
        cdhaek &= aekcdh+(q^4 - q^2)*afhceg+(1 - q^2)*bdkceg-(q^2 - 1)^2*bfgcdh,\\
        cdhafh &= afhcdh+(q^3 - q)*afhceg-(q^3 - q)*bfgcdh,\\
        cdhbdk &= bdkcdh-(q - 1/q)*bdkceg+(q - 1/q)*bfgcdh,
        \label{apeq:2}
    \end{split}
\end{equation}
with $bfg$ segment:
\begin{equation}
    \begin{split}
        bfgaek &= aekbfg+(q^4 - q^2)*afhceg+(1 - q^2)*bdkceg-(q^2 - 1)^2*bfgcdh,\\
        bfgafh &= afhbfg+(q^3 - q)*afhceg-(q^3 - q)*bfgcdh,\\
        bfgbdk &= bdkbfg-(q - 1/q)*bdkceg+(q - 1/q)*bfgcdh.
        \label{apeq:3}
    \end{split}
\end{equation}
The key observation is that when we switch the order of a high-complexity segment with a low-complexity segment, the newly generated monomials contain at most one high-complexity segment.

\hfill

\noindent When we switch the order of two high complexity segments:
\begin{equation}
    \begin{split}
        bdkafh =& q^{-2}*afhbdk+(1 - q^{-2})*aekbfg\\
        &+(1 - q^{-2})*aekcdh-(q^2 - 1)^2/q^3*aekceg\\
        &+\frac{(q^2 - 1)^2(q^2 + 1)}{q^2}*afhceg-(q^4 - q^2)*bfgcdh,
        \label{apeq:4}
    \end{split}
\end{equation}
\begin{equation}
    \begin{split}
        afhaek =& aekafh+(q - 1/q)*afhbdk-(q - 1/q)*aekbfg\\
        &-(q - 1/q)*aekcdh+(q - 1/q)^2*aekceg+(q - 1/q)*afhceg,\\
        \label{apeq:5}
    \end{split}
\end{equation}
\begin{equation}
    \begin{split}
        bdkaek =& aekbdk-(q - 1/q)*afhbdk+(q - 1/q)*aekbfg\\
        &+(q - 1/q)*aekcdh-(q - 1/q)^2*aekceg\\
        &+\frac{(q^2 - 1)^2(q^2 + 1)}{q}*afhceg-(q^3 - q)*bdkceg\\
        &-q(q^2 - 1)^2*bfgcdh.
        \label{apeq:6}
    \end{split}
\end{equation}
In Equation~(\ref{apeq:4}), the newly generated monomials contain at most one high-complexity segment. In Equation~(\ref{apeq:5}) and Equation~(\ref{apeq:6}), the newly generated monomials contain at most one high-complexity segment except the monomial $afhbdk$.

\hfill

\noindent Standard monomials $afhbdkceg$, $bdkafhceg$ and $aekbfgcdh$ have the same counting matrix:
\begin{equation*}
    \begin{bmatrix}
    1&1&1\\
    1&1&1\\
    1&1&1
    \end{bmatrix}.
\end{equation*}
We have the following equation:
\begin{equation}
    \begin{split}
        afhbdkceg =& q*aekbfgcdh+(1 - q^2)*aekbfgceg\\
        &+(1 - q^2)*aekcdhceg+(q^2 - 1)^2/q*aek(ceg)^2\\
        &+(1 - q^2)*afhbfgcdh+(q^3 - q)*afhbfgceg\\
        &+(q^3 - q)*afhcdhceg-(q^2 - 1)^2*afh(ceg)^2.
        \label{apeq:7}
    \end{split}
\end{equation}
\begin{equation}
    \begin{split}
        bdkafhceg =& 1/q*aekbfgcdh-(1 - q^{-2})*afhbfgcdh\\
        &+(q - q^{-1})*afhbfgceg+(q - q^{-1})*afhcdhceg\\
        &+(q^2 - 1)^2*afh(ceg)^2-(q^4 - q^2)*bfgcdh(ceg)^2.
        \label{apeq:8}
    \end{split}
\end{equation}
