# Supplementary material for: Computing the Haar state of $\mathcal{O}(SL_q(3))$ using value preserving (anti)homomorphisms
Source: arXiv:2401.08614 source file (2024-04-26)
Supplement: Supplementary file 2 [file appendix_E.tex]

\section{Example of $q$-Deformed Weingarten Function} \label{apd:e}
We know that when $q\rightarrow 1$, $\mathcal{O}(SU_q(n))$ becomes $SU(n)$ and the Haar state on $SU_q(n)$ becomes the Haar measure on $SU(n)$. This implies that 
\begin{equation*}
\begin{split}
    {\small h(x_{i_1j_1}\cdots x_{i_nj_n}x_{i_1'j_1'}^*\cdots x_{i_n'j_n'}^*)
    \xrightarrow{q\rightarrow 1}
    \int_{SU(n)}U_{i_1j_1}\cdots U_{i_nj_n}U_{i_1'j_1'}^*\cdots U_{i_n'j_n'}^*\ dU},
\end{split}
\end{equation*}
where $x_{i,j}$'s are generators of $\mathcal{O}(SU_q(n))$ and $U_{i,j}$'s are coordinate function on $SU(n)$. The Haar state on the quantum sphere serves as an example of $q$-deformed Weingarten function on $SU(n)$(for detail, see Noumi \textit{et al.}~\cite{noumi1993finite}, Reshetikhin \textit{et al.}~\cite{reshetikhin2001quantum}, Mikkelsen \textit{et al.}~\cite{mikkelsen2022haar}).

\hfill

\noindent One major difference between the Haar state and the integral is that the order of generators affects the Haar state. However, the order of the coordinate functions does not affect the integral. In the following examples on $\mathcal{O}(SU_q(3))$, we show that the order of generators in the Haar state does not affect the limit at $q=1$.

\hfill

\noindent \textbf{Example 1:}
\begin{equation*}
\begin{split}
h(x_{11}x_{22}x_{11}^*x_{22}^*)&=h(aea^*e^*)=h(ae(ek-q\cdot fh)(ak-q\cdot cg))\\
    &=h(aeekak)-q\cdot h(aefhak)-q\cdot h(aeekcg)+q^2\cdot h(aefhcg)\\
    &\frac{q^2}{(q^2+1)^2(q^4+1)}.
\end{split}
\end{equation*}
\begin{equation*}
    \begin{split}
h(x_{22}x_{11}x_{11}^*x_{22}^*)&=h(eaa^*e^*)=h(ea(ek-q\cdot fh)(ak-q\cdot cg))\\ 
    &=h(eaekak)-q\cdot h(eafhak)-q\cdot h(eaekcg)+q^2\cdot h(eafhcg)\\
    &=\frac{q^2}{(q^2+1)^2(q^4+1)}\frac{q^6+q^2+1}{q^4+q^2+1}
    \end{split}.
\end{equation*}
\begin{equation*}
    \begin{split}
        h(x_{11}x_{22}x_{22}^*x_{11}^*)&=h(aee^*a^*)=h(ae(ak-q\cdot cg)(ek-q\cdot fh))\\
        &=h(aeakek)-q\cdot h(aecgek)-q\cdot h(aeakfh)+q^2\cdot h(aecgfh)\\
        &=\frac{1}{(q^2+1)^2(q^4+1)}\frac{q^6+q^4+1}{q^4+q^2+1}.
    \end{split}
\end{equation*}
\begin{equation*}
    \begin{split}
        h(x_{11}x_{11}^*x_{22}x_{22}^*)&=h(aa^*ee^*)=h((aek-q\cdot afh)(eak-q\cdot ceg))\\
        &=h(aekeak)-q\cdot h(aekceg)-q\cdot h(afheak)+q^2\cdot h(afhceg)\\
       &=\frac{q^2}{(q^2+1)^2(q^4+1)}.
    \end{split}
\end{equation*}
The Haar states of monomials in other orders can be computed by the relation $h(y\phi(x))=h(xy)$ where $\phi$ is the homomorphism on $\mathcal{O}(SU_q(3))$ such that $\phi(x_{ij})=q^{2(i+j-4)}x_{ij}$. When $q\rightarrow 1$, all Haar state values goes to $1/8$ which is consistent with 
\begin{equation*}
    \int_{SU(3)}U_{11}U_{22}U_{11}^*U_{22}^*\ dU=Wg(1^2,3)=\frac{1}{3^2-1}=\frac{1}{8}.
\end{equation*}
\textbf{Example 2:}
\begin{equation*}
    \begin{split}
        h(x_{11}x_{32}x_{31}^*x_{12}^*)&=h(ahg^*b^*)=(-q)^{-1}\cdot h(ah(bf-q\cdot ce)(dk-q\cdot fg))\\
        &=-q^{-1}[h(ahbfdk)-q\cdot h(ahcedk)-q\cdot h(ahbffg)+q^2\cdot h(ahcefg)]\\
        &=\frac{-q}{(q^2+1)^2(q^4+1)(q^4+q^2+1)}.
    \end{split}
\end{equation*}
\begin{equation*}
    \begin{split}
        h(x_{32}x_{11}x_{31}^*x_{12}^*)&=h(hag^*b^*)=(-q)^{-1}\cdot h(ha(bf-q\cdot ce)(dk-q\cdot fg))\\
        &=-q^{-1}[h(habfdk)-q\cdot h(hacedk)-q\cdot h(habffg)+q^2\cdot h(hacefg)]\\
        &=\frac{-q^7}{(q^2+1)^2(q^4+1)(q^4+q^2+1)}.
    \end{split}
\end{equation*}
\begin{equation*}
    \begin{split}
        h(x_{11}x_{32}x_{12}^*x_{31}^*)&=h(ahb^*g^*)=(-q)^{-1}\cdot h(ah(dk-q\cdot fg)(bf-q\cdot ce))\\
        &=-q^{-1}[h(ahdkbf)-q\cdot h(ahdkce)-q\cdot h(ahfgbf)+q^2\cdot h(ahfgce)]\\
        &=\frac{-q}{(q^2+1)^2(q^4+1)(q^4+q^2+1)}.
    \end{split}
\end{equation*}
\begin{equation*}
    \begin{split}
        h(x_{11}x_{12}^*x_{32}x_{31}^*)&=h(ab^*hg^*)=(-q)^{-1}\cdot h(a(dk-q\cdot fg)h(bf-q\cdot ce))\\
        &=-q^{-1}[h(adkhbf)-q\cdot h(adkhce)-q\cdot h(afghbf)+q^2\cdot h(afghce)]\\
        &=\frac{-q^4}{(q^2+1)^2(q^4+1)(q^4+q^2+1)}.
    \end{split}
\end{equation*}
When $q\rightarrow 1$, all Haar state values goes to $-1/24$ which is consistent with 
\begin{equation*}
    \int_{SU(3)}U_{11}U_{32}U_{31}^*U_{12}^*\ dU=Wg(2,3)=-\frac{1}{3(3^2-1)}=-\frac{1}{24}.
\end{equation*}
\textbf{Example 3:}
\begin{equation*}
    \begin{split}
        h(x_{11}x_{11}x_{11}^*x_{11}^*)&=h(aaa^*a^*)=h(aa(ek-q\cdot fh)(ek-q\cdot fh))\\
        &=h(aaekek)-q\cdot h(aafhek)-q\cdot h(aaekfh)+q^2\cdot h(aafhfh)\\
        &=\frac{1}{(q^4+1)(q^4+q^2+1)}.
    \end{split}
\end{equation*}
\begin{equation*}
    \begin{split}
        h(x_{11}x_{11}^*x_{11}x_{11}^*)&=h(aa^*aa^*)=h(a(ek-q\cdot fh)a(ek-q\cdot fh))\\
        &=h(aekaek)-q\cdot h(afhaek)-q\cdot h(aekafh)+q^2\cdot h(afhafh)\\
        &=\frac{q^4-q^2+1}{(q^4+1)(q^4+q^2+1)}.
    \end{split}
\end{equation*}
When $q\rightarrow 1$, all Haar state values goes to $1/6$ which is consistent with 
\begin{equation*}
\begin{split}
    \int_{SU(3)}U_{11}^2(U_{11}^*)^2\ dU&=2Wg(1^2,3)+2Wg(2,3)\\
    &=2\frac{1}{3^2-1}-2\frac{1}{3(3^2-1)}=\frac{1}{6}.
\end{split}  
\end{equation*}
