# Supplementary material for: Computing the Haar state of $\mathcal{O}(SL_q(3))$ using value preserving (anti)homomorphisms
Source: arXiv:2401.08614 source file (2024-04-26)
Supplement: Supplementary file 5 [file appendix_D.tex]

\section{Illustration of the Zigzag Recursive Relation} \label{apd:d}

\tikzstyle{smallbox} = [rectangle,  minimum width=0.5cm, minimum height=0.5cm, text centered, draw=white, fill=white!100]
\tikzstyle{box} = [rectangle, minimum width=3.7cm, minimum height=1cm, text centered, draw=black, fill=white!100]
\tikzstyle{arrow} = [thick,->,>=stealth]
\tikzstyle{arrow_v} = [thick,->,>=stealth, double distance=1pt]

\begin{figure}[htb!]
\centering
\resizebox{0.75\textwidth}{!}{

\begin{tikzpicture}
\node (label1) [smallbox] {\rotatebox{180}{$\mathbf{\vdots}$}};
\node (label2) [smallbox, right of=label1, xshift= 5cm]   {\rotatebox{180}{$\mathbf{\vdots}$}};
\node (label3) [box, below of=label1, yshift= -0.8cm]      {$bfg(cdh)^{j-1}(ceg)^{n-j+1}$};
\node (label4) [box, right of=label3, xshift= 5cm]      {$bdk(cdh)^{j-1}(ceg)^{n-j+1}$};
\node (label5) [box, below of=label3, yshift= -0.8cm]      {$bfg(cdh)^{j}(ceg)^{n-j}$};
\node (label6) [box, right of=label5, xshift= 5cm]      {$bdk(cdh)^{j}(ceg)^{n-j}$};
\node (label7) [box, below of=label5, yshift= -0.8cm]      {$bfg(cdh)^{j+1}(ceg)^{n-j-1}$};
\node (label8) [box, right of=label7, xshift= 5cm]      {$bdk(cdh)^{j+1}(ceg)^{n-j-1}$};
\node (label9) [smallbox, below of=label7, yshift= -0.8cm]      {\rotatebox{0}{$\mathbf{\vdots}$}};
\node (label10) [smallbox, right of=label9, xshift= 5cm]      {\rotatebox{0}{$\mathbf{\vdots}$}};

\draw [arrow_v] (label1) -- node[anchor=east] {1} (label3);
\draw [arrow_v] (label3) -- node[anchor=east] {3} (label5);
\draw [arrow_v] (label5) -- node[anchor=east] {5} (label7);
\draw [arrow_v] (label7) -- node[anchor=east] {7} (label9);

\draw [arrow_v] (label2) -- node[anchor=west] {2} (label4);
\draw [arrow_v] (label4) -- node[anchor=west] {4} (label6);
\draw [arrow_v] (label6) -- node[anchor=west] {6} (label8);
\draw [arrow_v] (label8) -- node[anchor=west] {8} (label10);

\draw [arrow] (label3) -- node[anchor=south] {} (label4);
\draw [arrow] (label5) -- node[anchor=south] {} (label6);
\draw [arrow] (label7) -- node[anchor=south] {} (label8);

\draw [arrow] (label4) -- node[anchor=south, xshift=-0.1cm, yshift=-0.1cm] {\rotatebox{30}{}} (label5);
\draw [arrow] (label6) -- node[anchor=south, xshift=-0.1cm, yshift=-0.1cm] {\rotatebox{30}{}} (label7);

\end{tikzpicture}
}
\caption{Illustration of the Zigzag recursive relation. Arrow 1 to 8 means that we are using the monomial in the upper box as the equation basis and $(aek)^{m-1}afh$ as the comparing basis to derive the linear relation containing the monomial in the lower box as the only unknown. The zigzagging arrows indicate the order that we follow to solve the Haar states of these monomials. }
\label{fig:my_label}
\end{figure}
